# Supplementary material for: MotionScape: A Motion-Stratified UAV Video Benchmark for World Modeling and Future Video Generation
Source: arXiv:2604.07991 source file (2026-09-08)
Supplement: Supplementary file 1 [file supplement.tex]

\documentclass[11pt]{article}

\usepackage[utf8]{inputenc}
\usepackage[T1]{fontenc}
\usepackage{lmodern}
\usepackage{geometry}
\usepackage{graphicx}
\usepackage{booktabs}
\usepackage{multirow}
\usepackage{amsmath, amssymb}
\usepackage{hyperref}
\usepackage{xcolor}
\usepackage{caption}
\usepackage{subcaption}

\geometry{a4paper, margin=1in}

\title{Supplementary Material}
\author{Anonymous}
\date{}

\begin{document}

\maketitle

\section{Additional Dataset Statistics}
\subsection{Resolution Distribution}
Add more detailed resolution statistics here.

\subsection{Scene Distribution}
Add scene category statistics here.

\subsection{Weather Distribution}
Add weather category statistics here.

\section{Experiment Details}
\subsection{ CLIP-based Coarse Filtering.}
prompt

\subsection{Semantic Annotation.}
In the semantic annotation stage, we carefully design the prompt so that the generated caption is primarily used to accurately describe the UAV's camera motion trend, while environment-related information is stored separately in the environment field. This avoids mixing excessive static scene descriptions into motion descriptions, thereby reducing semantic redundancy and making the caption more focused on viewpoint changes, which better matches the needs of downstream viewpoint-controllable generation tasks. The specific prompt used in the semantic annotation stage is presented below; note that it does not include the prompt used for irrelevant-content filtering.

You are provided RGB image frame.
Analyze the weather, environment, drone maneuver, and provide a detailed video caption.

TASK: SCENE ANALYSIS

[Weather Categories]

- Sunny / Overcast / Rainy / Snowy / Fog/Haze / Night / Indoor / Unknown
  
Please output the result in STRICT JSON format with the following keys:
{
  "weather": "Select from Weather Categories (or 'N/A' if false)",
  
  "environment": "Brief description of the scene, max 5 words (or 'N/A')",
  
  "caption": "Write a detailed 2-3 sentence objective caption of the target video segment for controllable video generation. The first sentence should describe the scene type, environmental layout, lighting, and weather conditions. The remaining sentences should describe the drone camera motion in a precise and structured way. The motion description must explicitly specify the flight direction, trajectory, motion speed or speed change, camera rotation direction and type, viewpoint changes, and, when relevant, the drone's relative motion with respect to the surrounding terrain or scene structure (e.g., maintaining altitude over descending terrain, moving through dense trees, or revealing a wider landscape). Use concrete motion terms such as forward motion, left turn, right turn, ascent, descent, yaw, pitch, tilt, acceleration, deceleration, and viewpoint expansion when appropriate. Keep the description factual, concise, and motion-oriented. Do not use subjective, emotional, aesthetic, or cinematic language such as 'beautiful', 'serene', 'dramatic', 'graceful', or 'evoking'. (or 'N/A')"
}

\section{Additional Results}
\subsection{Qualitative Results}
In the main paper, we present quantitative results under three different conditioning settings to analyze model behavior in high-dynamic UAV video continuation. In this section, we further provide the corresponding qualitative results and show the prompt associated with each conditioning setting. These comparisons reveal that even a strong baseline such as Cosmos 2.5-2B still struggles to consistently follow conditioning instructions in this scenario, with clear limitations in viewpoint control, motion trend preservation, and temporal coherence. This further suggests that high-dynamic aerial scenes pose a more stringent challenge to current world models and also highlights the value of our dataset for evaluating such capabilities.

\end{document}
